# Supplementary material for: Spatio-Temporal Analysis of Surveillance Data
Source: arXiv:1711.00555 ancillary file (2017-11-01)
Supplement: Supplementary file 1 [file SurveillanceChapterArxiv_supp.pdf]

# Supplementary Materials for "Spatio-Temporal Analysis of Surveillance Data"

Jon Wakefield, Tracy Dong and Vladimir Minin

## 1 Analysis of Measles Data

We analyze the weekly measles incidence data in 17 districts of the Weser-Ems region of Lower Saxony in Germany from 2001 to 2002 by fitting a TSIR model and an epidemic/endemic model.

### 1.1 Fitting the TSIR Model

We fit the following TSIR model using the `rstan` package.

$$
\begin{aligned}
Y_{it}|\mu_{it} &\sim \text{NegBin}\left(\mu_{it}, \phi\right) \\
\mu_{it} &= \left[ \mathsf{e}^{\lambda_t^{\text{AR}}} y_{i,t-1} + \mathsf{e}^{\lambda^{\text{NE}}} N_i^{\tau_1} \sum_{j=1}^{n} w_{ij} y_{j,t-1}^{\tau_2} \right]^{\alpha} + N_i \mathsf{e}^{\lambda^{\text{EN}}} \\
w_{ij} &= \frac{d_{ij}^{-\theta_1/(1-\theta_1)}}{\sum_{k \neq i} d_{ik}^{-\theta_1/(1-\theta_1)}} \\
\lambda_t^{\text{AR}} &= \beta_0^{\text{AR}} + \beta_1^{\text{AR}} t + \gamma \sin(\omega t) + \delta \cos(\omega t)
\end{aligned}
$$

Here, $d_{ij}$ is the distance between areas $i$ and $j$.

We use the following priors on $\theta_1$ and $\alpha$ and use flat priors for the rest of the parameters.

$$
\begin{aligned}
\theta_1 &\sim \text{Uniform}(0, 1) \\
\alpha &\sim \text{Uniform}(0.95, 1)
\end{aligned}
$$

We run a total of 6,000 iterations and use 3,000 posterior samples for parameter estimation after burn-in. Table 1 shows the posterior means and standard deviations of the parameters in the TSIR model.

| | Parameter | Posterior Mean | Posterior SD |
|---|---|---|---|
| 1 | $\beta_0^{\text{AR}}$ | -0.582 | 0.356 |
| 2 | $\beta_1^{\text{AR}}$ | 0.00073 | 0.00609 |
| 3 | $\gamma$ | 0.524 | 0.227 |
| 4 | $\delta$ | 0.104 | 0.170 |
| 5 | $\lambda^{\text{NE}}$ | 0.274 | 0.642 |
| 6 | $\lambda^{\text{EN}}$ | -0.424 | 0.217 |
| 7 | $\alpha$ | 0.976 | 0.014 |
| 8 | $\tau_1$ | 0.312 | 0.198 |
| 9 | $\tau_2$ | 0.329 | 0.133 |
| 10 | $\theta_1$ | 0.751 | 0.037 |
| 11 | $\phi$ | 2.075 | 0.284 |

Table 1: Posterior means and standard deviations of the parameters in the TSIR model.

## 1.2 Fitting the Epidemic/Endemic Model

We fit the following epidemic/endemic model using both the `rstan` package and the `surveillance` package.

$$
\begin{aligned}
Y_{it}|\mu_{it} &\sim \text{NegBin}(\mu_{it}, \phi) \\
\mu_{it} &= \text{e}^{\lambda^{\text{AR}} + b_i^{\text{AR}}} y_{i,t-1} + \text{e}^{\lambda^{\text{NE}} + b_i^{\text{NE}}} \sum_{j=1}^{n} w_{ij} y_{j,t-1} + N_i \text{e}^{\lambda_t^{\text{EN}} + b_i^{\text{EN}}} \\
w_{ij} &= \frac{m_{ij}^{-\theta_2/(1-\theta_2)}}{\sum_{k \neq i} m_{ik}^{-\theta_2/(1-\theta_2)}} = \frac{m_{ij}^{-\rho}}{\sum_{k \neq i} m_{ik}^{-\rho}} \\
\lambda_t^{\text{EN}} &= \beta_0^{\text{EN}} + \beta_1^{\text{EN}} t + \gamma \sin(\omega t) + \delta \cos(\omega t) \\
b_i^{\text{AR}} &\sim \text{Normal}(0, \sigma^2_{\text{AR}}) \\
b_i^{\text{EN}} &\sim \text{Normal}(0, \sigma^2_{\text{EN}}) \\
b_i^{\text{NE}} &\sim \text{Normal}(0, \sigma^2_{\text{NE}})
\end{aligned}
$$

Here, $m_{ij}$ is the number of boundaries to cross when traveling between areas $i$ and $j$.

We use a flat prior on $\phi$ and the following priors for the rest of the parameters.

$$\lambda^{\text{AR}} \sim \text{Normal}(0, 100)$$
$$\lambda^{\text{NE}} \sim \text{Normal}(0, 100)$$
$$\beta_0^{\text{EN}} \sim \text{Normal}(0, 100)$$
$$\beta_1^{\text{EN}} \sim \text{Normal}(0, 100)$$
$$\gamma \sim \text{Normal}(0, 100)$$
$$\delta \sim \text{Normal}(0, 100)$$
$$\theta_2 \sim \text{Uniform}(0, 1)$$
$$\sigma^2_{\text{AR}} \sim \text{Inverse Gamma}(0.5, 0.1)$$
$$\sigma^2_{\text{NE}} \sim \text{Inverse Gamma}(0.5, 0.1)$$
$$\sigma^2_{\text{EN}} \sim \text{Inverse Gamma}(0.5, 0.1)$$

We run a total of 10,000 iterations and use 6,000 posterior samples for parameter estimation after burn-in. Table 2 shows the point estimates and standard error estimates from the `surveillance` package, as well as the posterior means and standard deviations from the `rstan` package, for each parameter in the epidemic/endemic model.

| | Parameter | `hhh4` Estimate | `rstan` Posterior Mean | `hhh4` SE | `rstan` Posterior SD |
|---|---|---|---|---|---|
| 1 | $\sigma_{AR}$ | 1.024 | 1.357 | | |
| 2 | $\sigma_{NE}$ | 1.655 | 3.388 | | |
| 3 | $\sigma_{EN}$ | 1.368 | 1.599 | | |
| 4 | $\lambda^{AR}$ | -1.596 | -1.778 | 0.378 | 0.752 |
| 5 | $\lambda^{NE}$ | -2.591 | -4.867 | 0.488 | 1.709 |
| 6 | $\beta_0^{\text{EN}}$ | -0.544 | -0.835 | 0.459 | 0.537 |
| 7 | $\beta_1^{\text{EN}}$ | 0.00239 | 0.00647 | 0.00522 | 0.00539 |
| 8 | $\gamma$ | 0.997 | 1.145 | 0.232 | 0.239 |
| 9 | $\delta$ | -0.626 | -0.653 | 0.207 | 0.198 |
| 10 | $\theta_2(\rho)$ | 0.807 (4.193) | 0.652 (1.873) | (0.749) | 0.212 |
| 11 | $\phi$ | 0.972 | 1.195 | 0.150 | 0.180 |

Table 2: Point estimates and standard error estimates from the `surveillance` package, posterior means and standard deviations from the `rstan` package, for each parameter in the epidemic/endemic model.

## 1.3 Graphical Summaries of the Fitted Models

Figure 1 and Figure 2 show the histograms, density estimates and traceplots of the posterior marginals for the parameters in the TSIR model. Figure 3 shows the observed (black dots) data in the 15 districts

with non-zero counts, and posterior summaries (2.5%, 50%, 97.5% quantiles) for $\mu_{it}$, under the TSIR model. Figure 4 shows the standardized residuals (dark grey dots) for the 15 districts with non-zero counts under the TSIR model, where the standardized residual for area $i$ at time $t$ is calculated by $\frac{y_{i,t}-\hat{\mu}_{i,t}}{\sqrt{\hat{\mu}_{i,t}+\frac{\hat{\mu}_{i,t}^2}{\hat{\phi}}}}$.

Figure 5 and Figure 6 show the histograms, density estimates and traceplots of the posterior marginals for the parameters in the epidemic/endemic model. Figure 7 shows the observed (black dots) data in the 15 districts with non-zero counts, and posterior summaries (2.5%, 50%, 97.5% quantiles) for $\mu_{it}$, under the epidemic/endemic model. Figure 8 shows the standardized residuals (dark grey dots) for the 15 districts with non-zero counts under the epidemic/endemic model, where the standardized residual for area $i$ at time $t$ is calculated by $\frac{y_{i,t}-\hat{\mu}_{i,t}}{\sqrt{\hat{\mu}_{i,t}+\frac{\hat{\mu}_{i,t}^2}{\hat{\phi}}}}$. Figure 9 shows the posterior medians of the autoregressive, neighborhood and endemic random effects $b_i^{\mathsf{AR}}$, $b_i^{\mathsf{NE}}$ and $b_i^{\mathsf{EN}}$ in the epidemic/endemic model.

Figure 10 shows the posterior medians of $\mu_{it}$ under the epidemic/endemic model and the TSIR model in the 15 districts with non-zero counts.

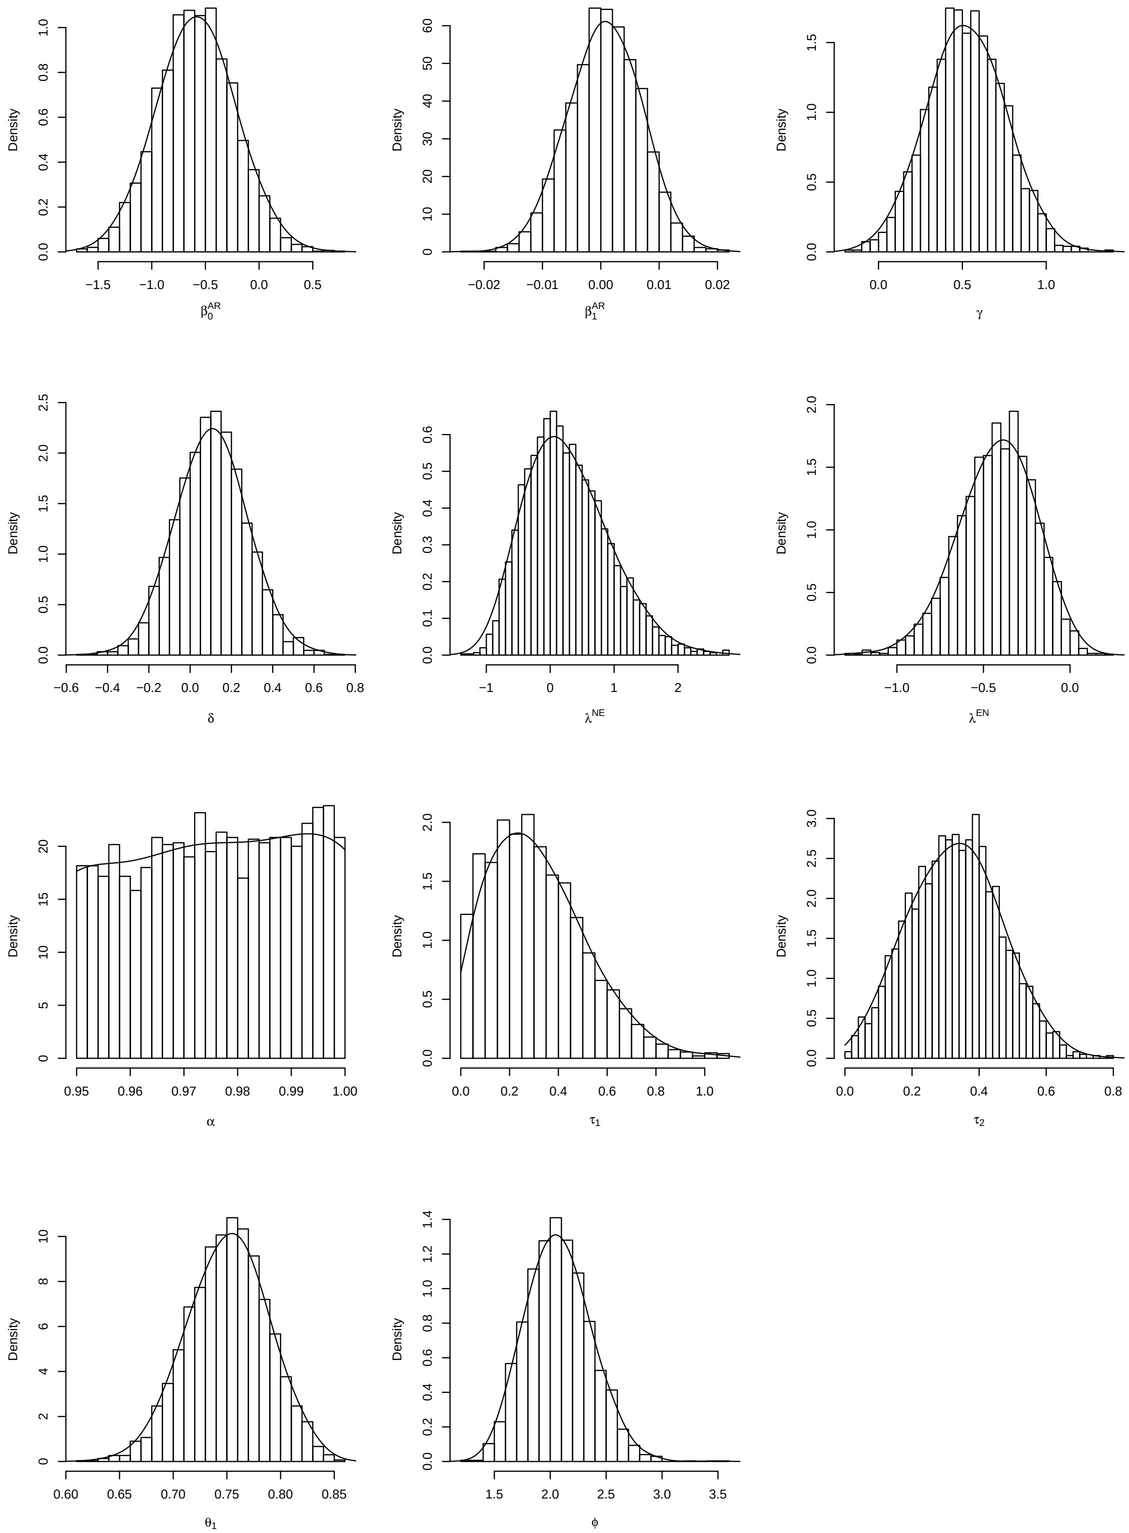


Figure 1: Posterior density for each parameter in the TSIR model.

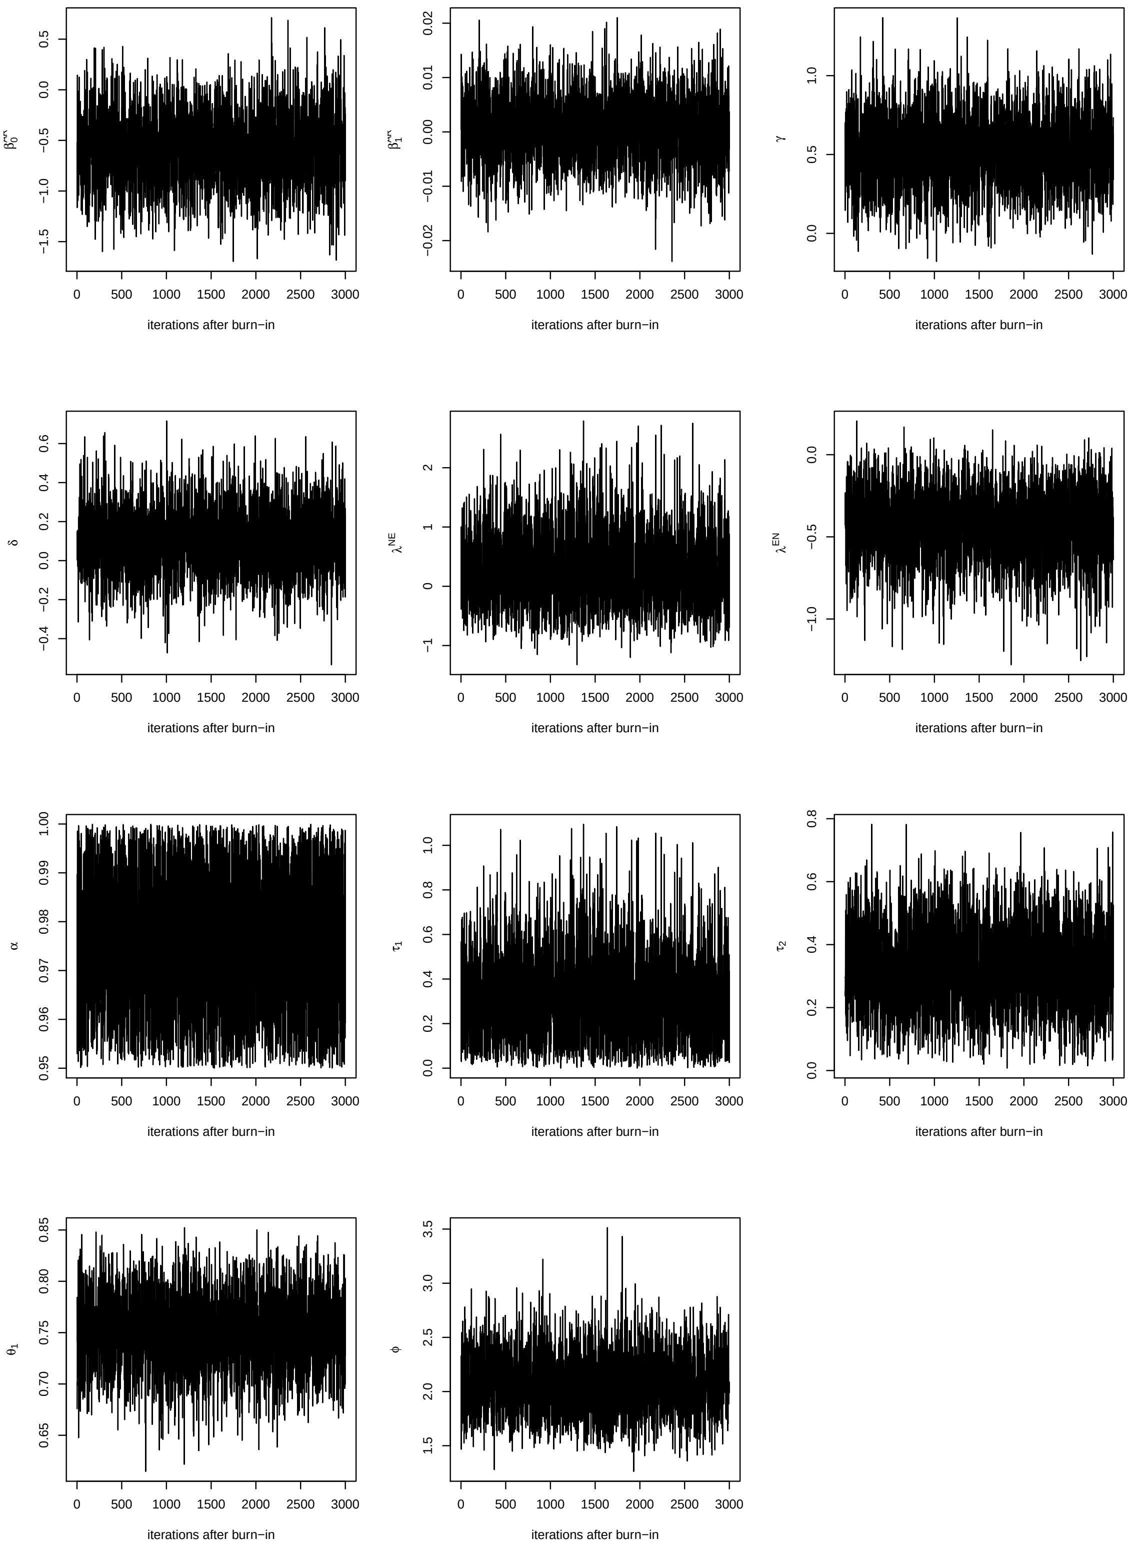


Figure 2: Posterior traceplot for each parameter in the TSIR model.

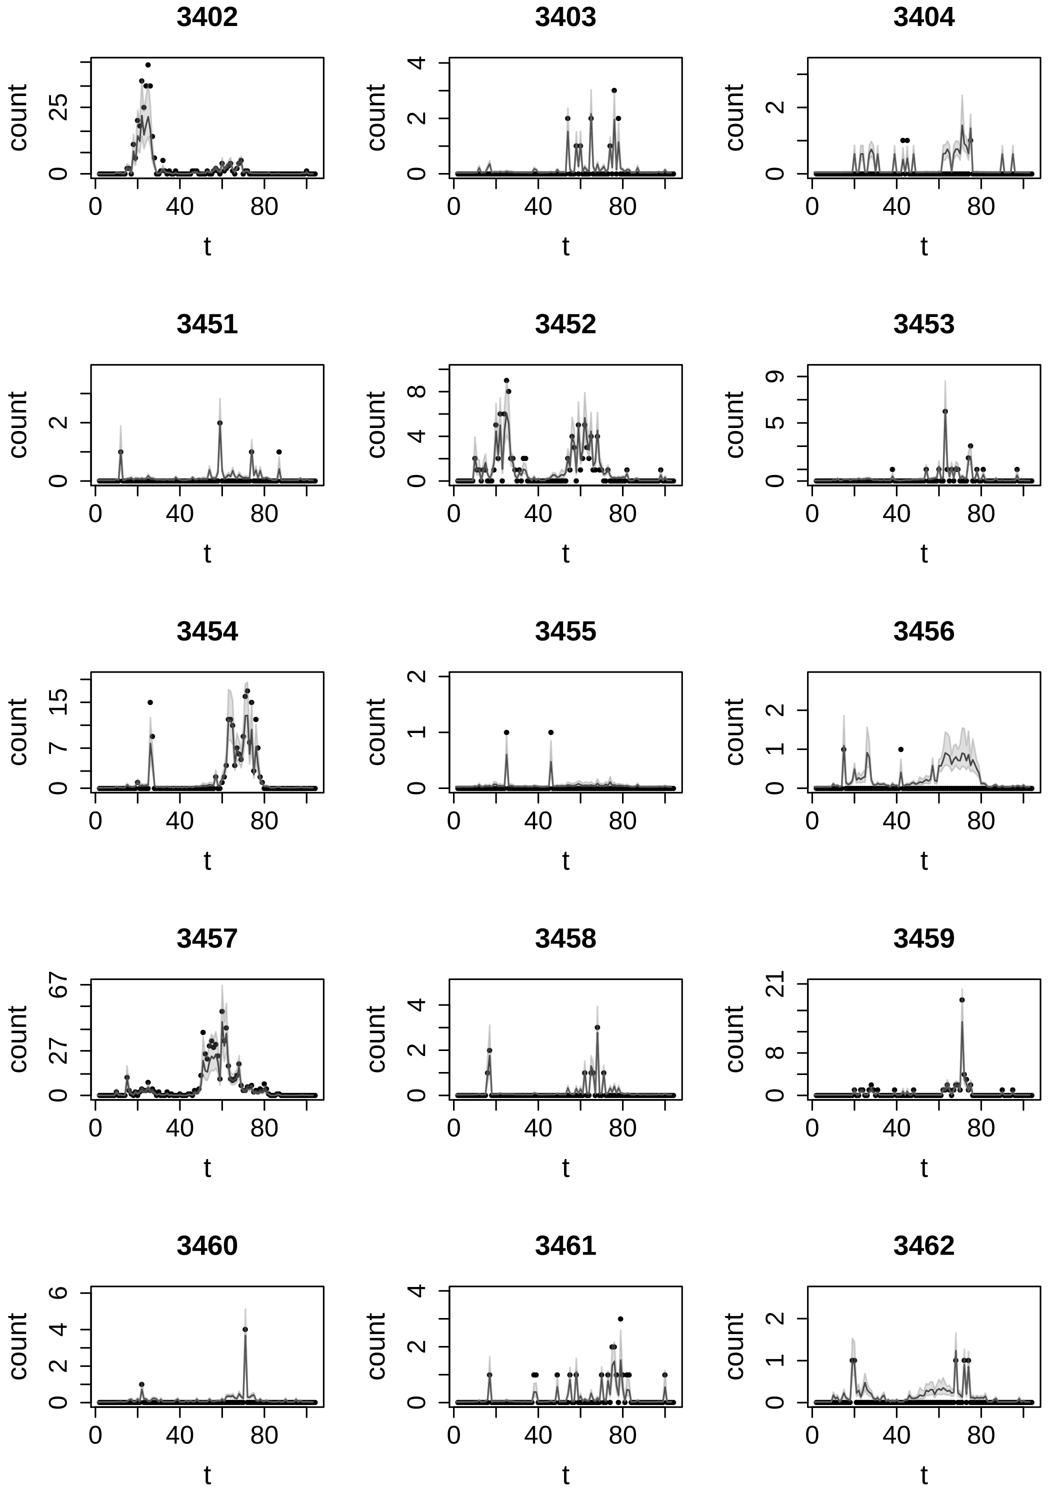


Figure 3: Observed (black dots) data in the 15 districts with non-zero counts, and posterior summaries (2.5%, 50%, 97.5% quantiles) for $\mu_{it}$, under the TSIR model.

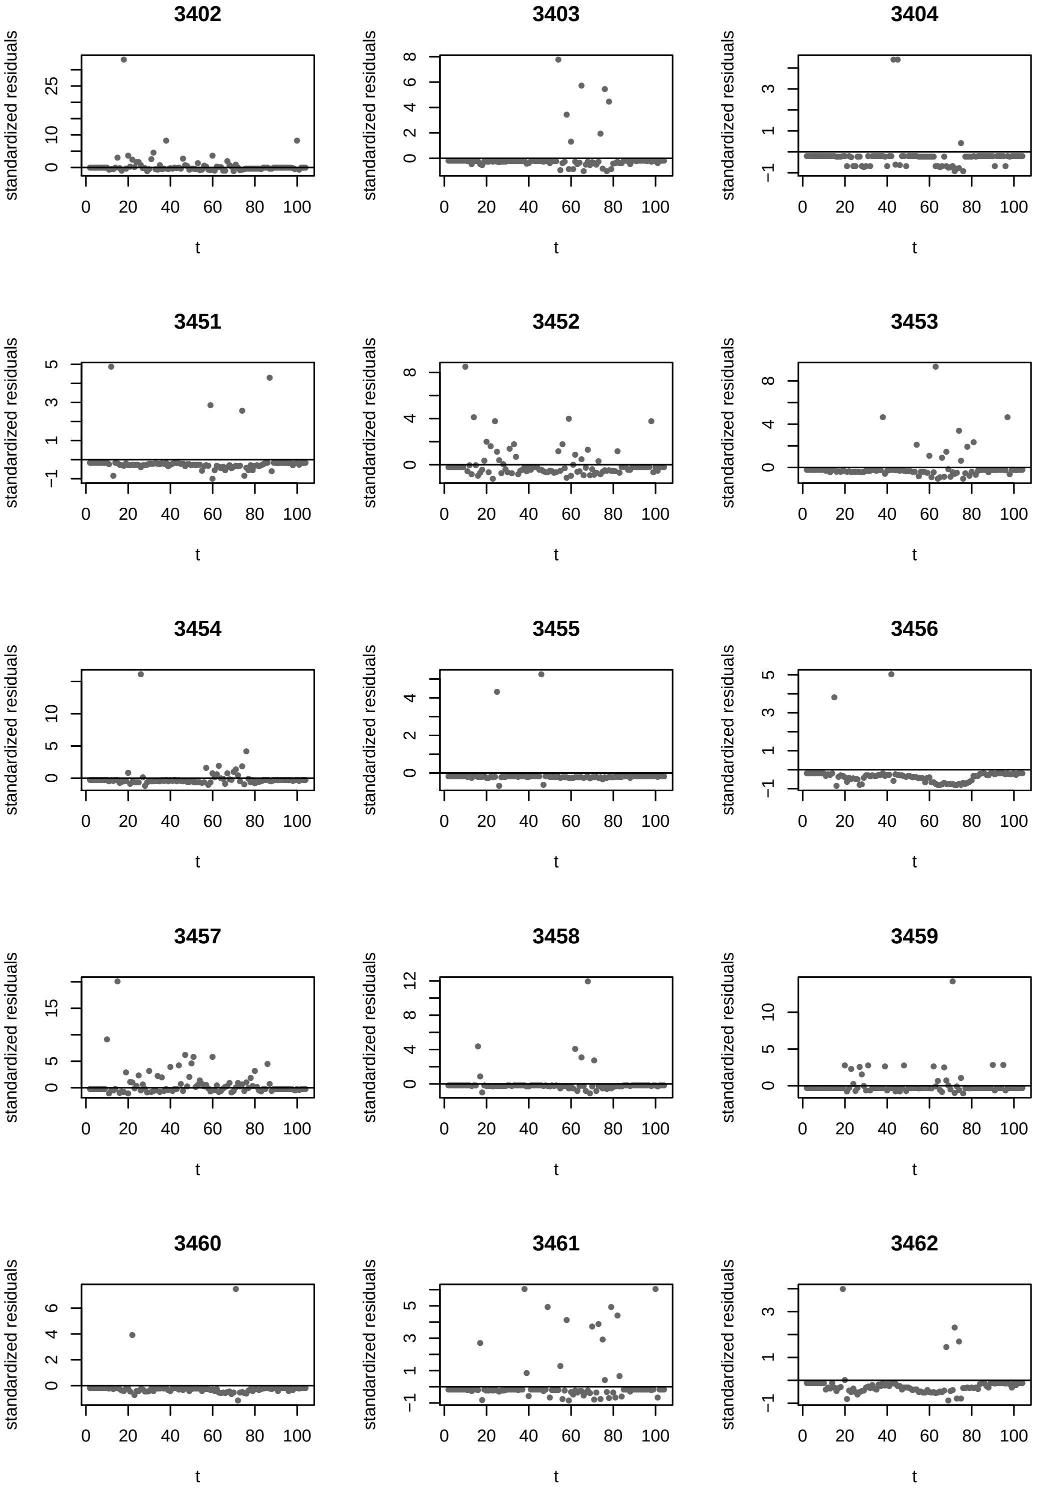


Figure 4: Standardized residuals (dark grey dots) for the 15 districts with non-zero counts under the TSIR model.

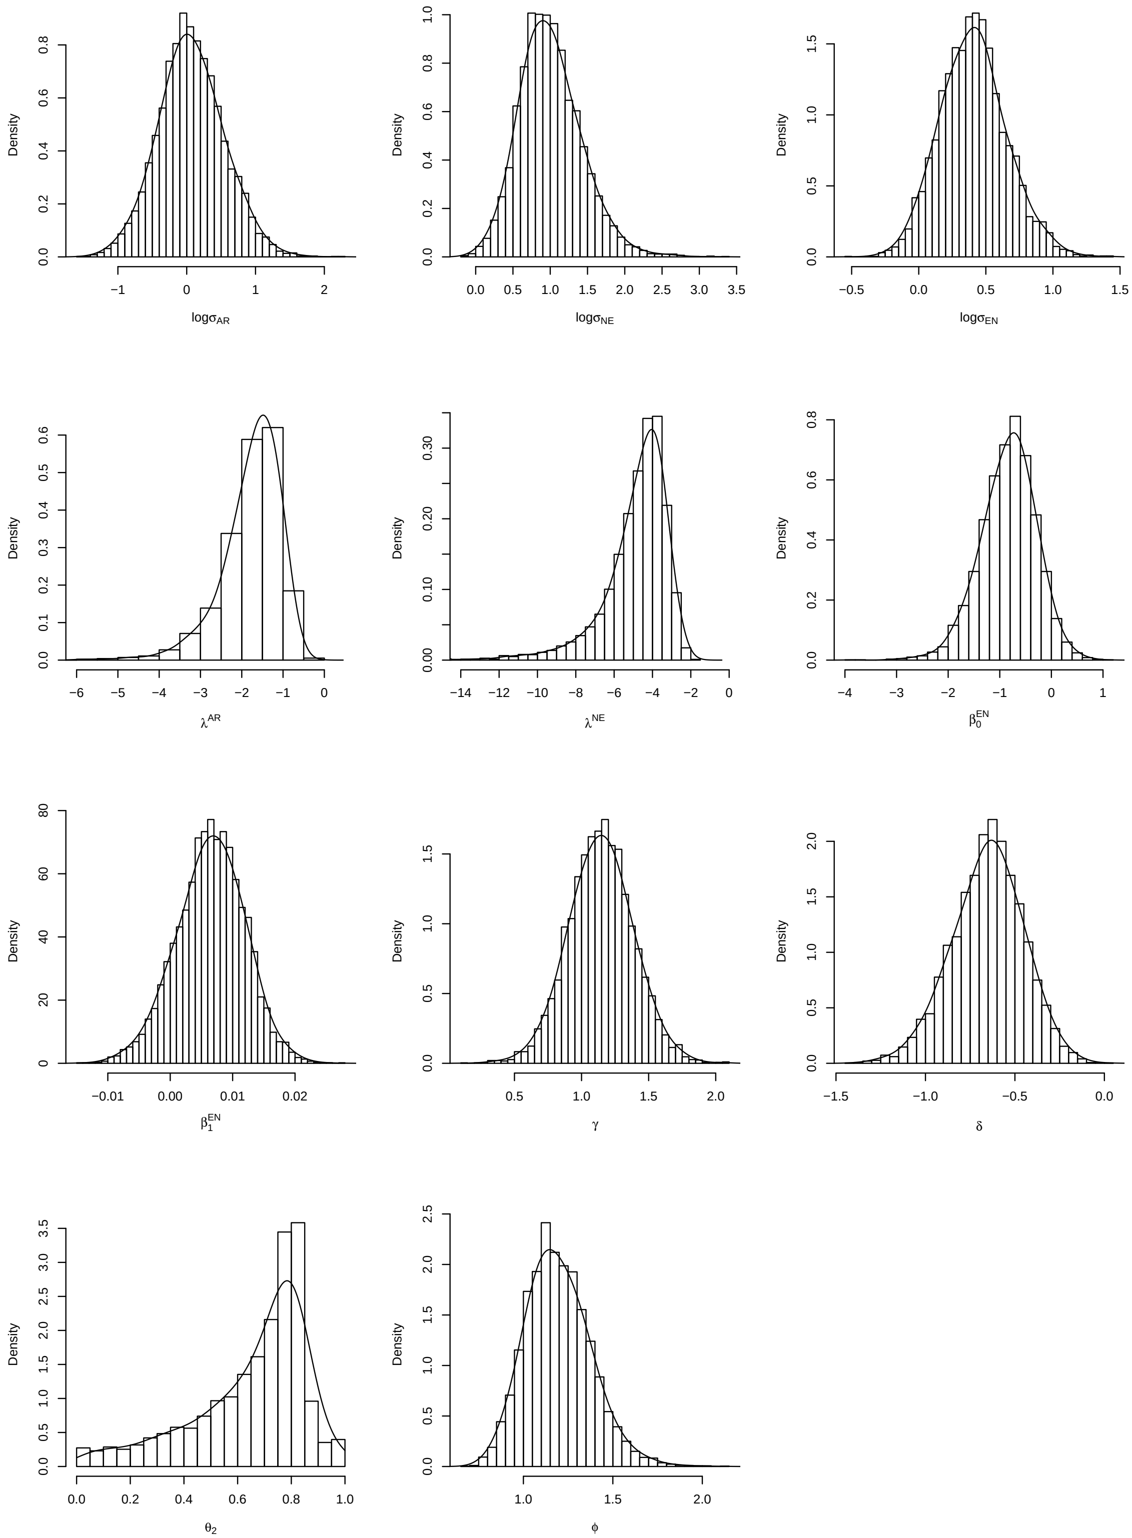


Figure 5: Histograms and density estimates of the posterior marginals for each parameter in the epidemic/endemic model.

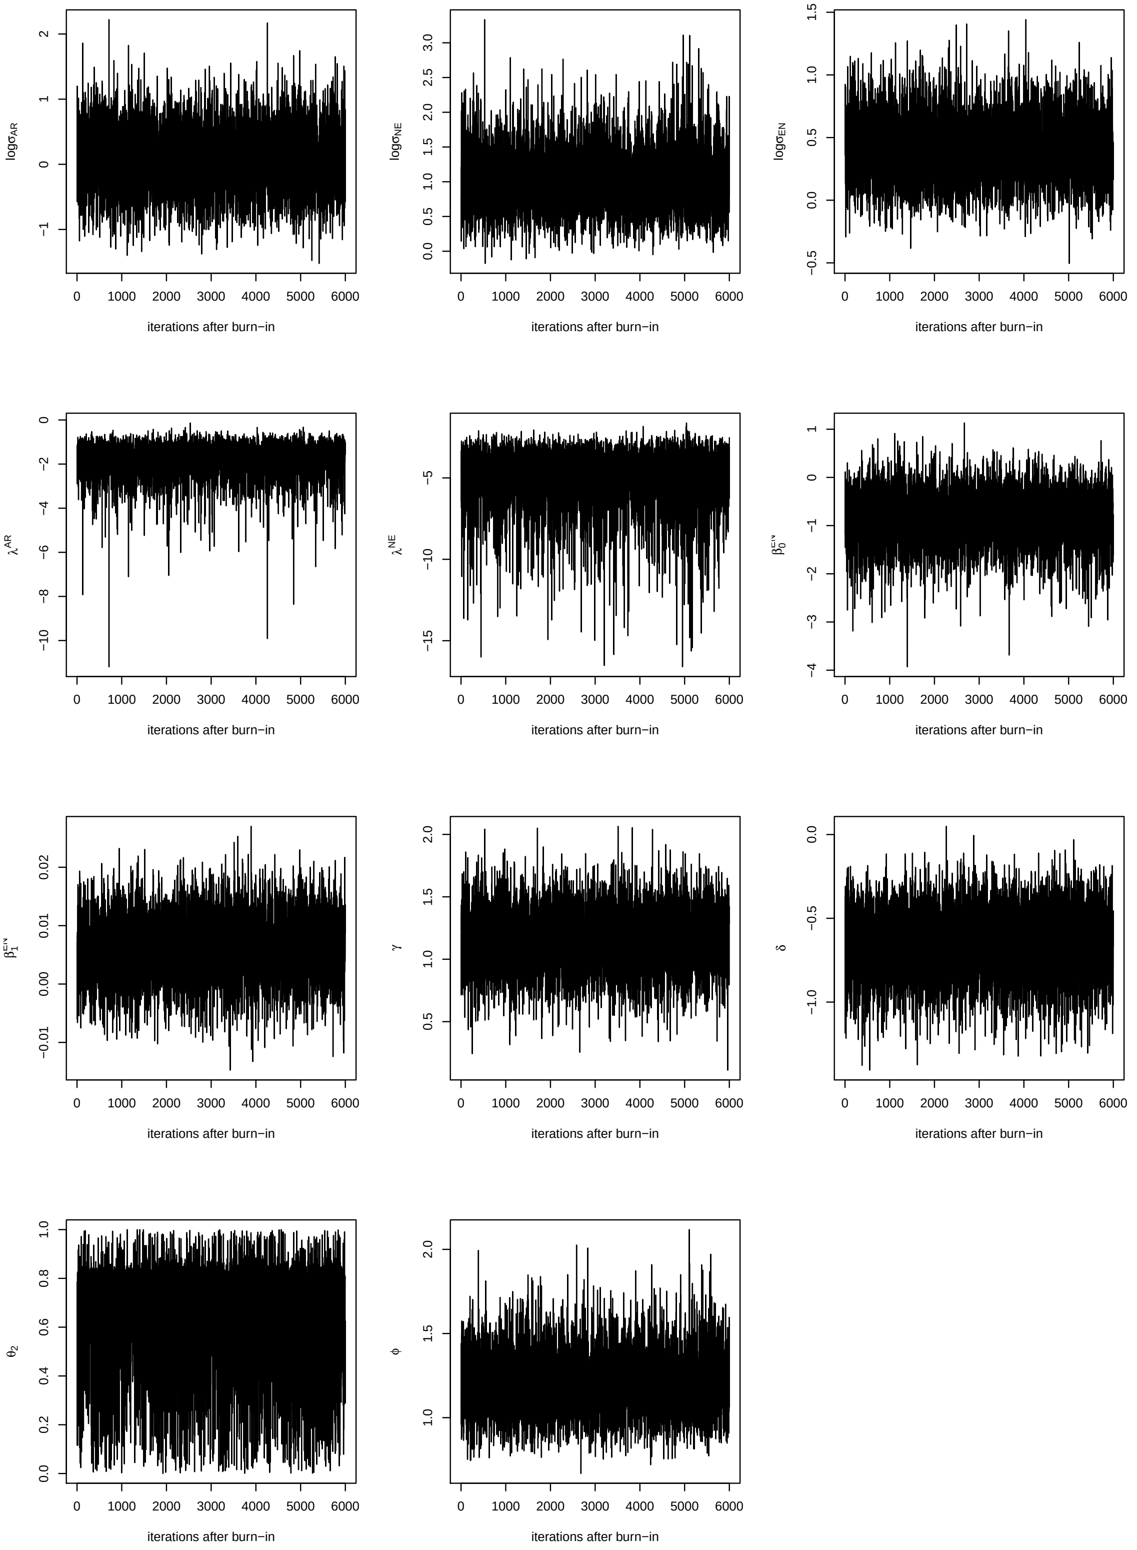


Figure 6: Posterior traceplot for each parameter in the epidemic/endemic model.

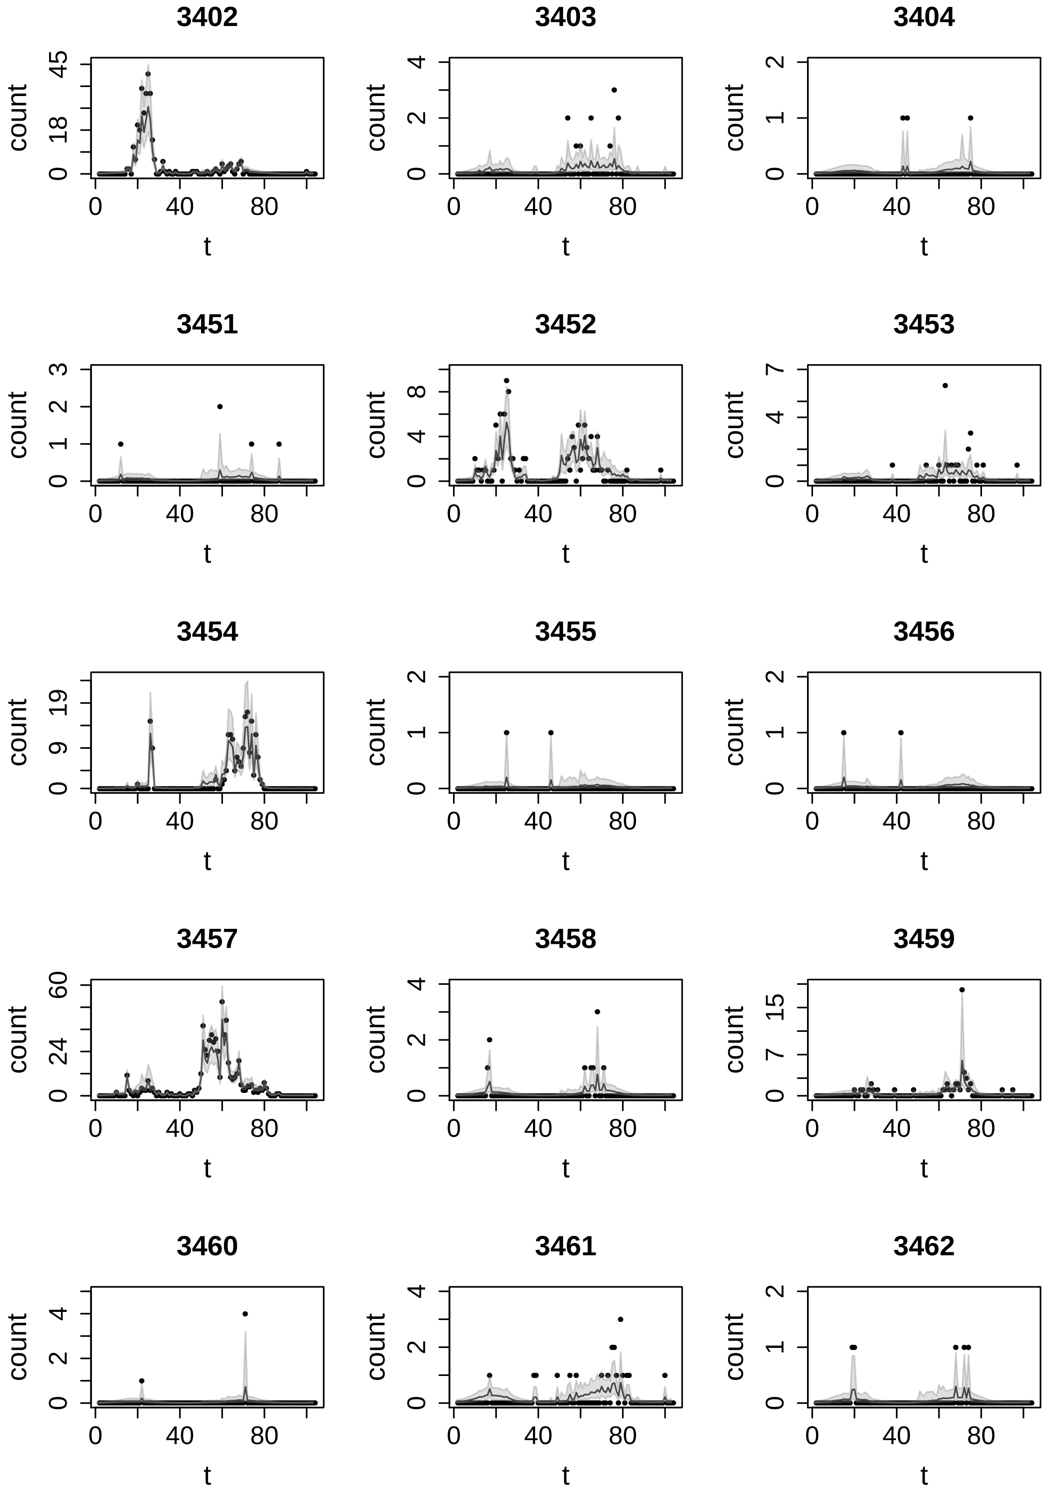


Figure 7: Observed (black dots) data in the 15 districts with non-zero counts, and posterior summaries (2.5%, 50%, 97.5% quantiles) for $\mu_{it}$, under the epidemic/endemic model.

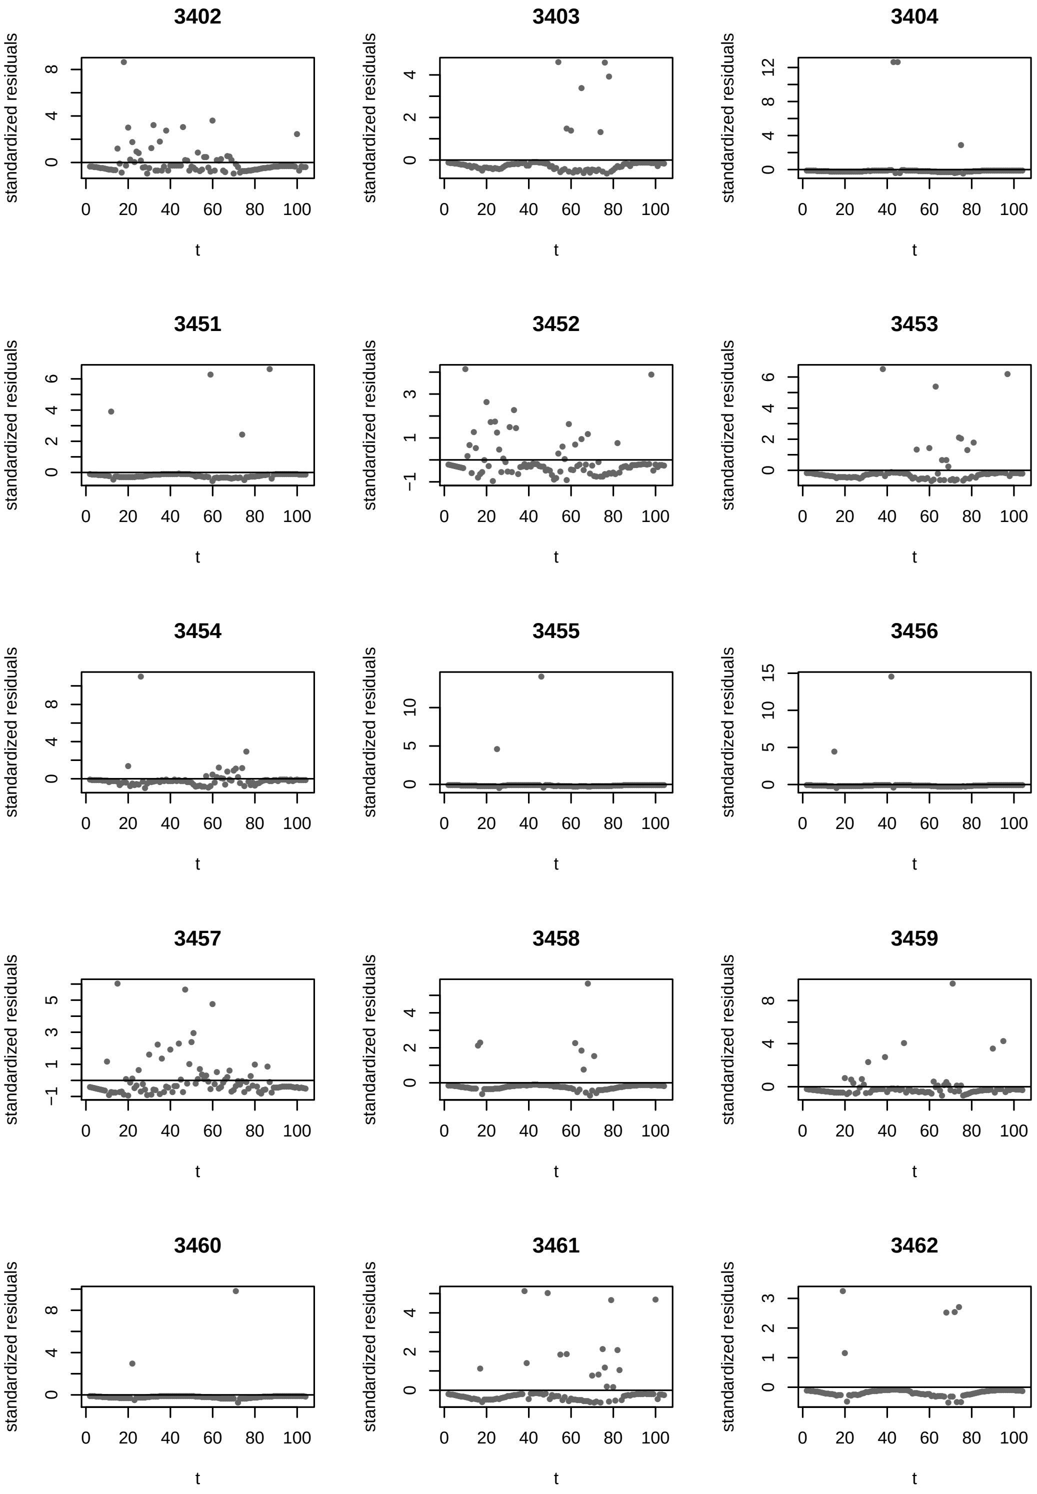


Figure 8: Standardized residuals (dark grey dots) for the 15 districts with non-zero counts under the epidemic/endemic model.

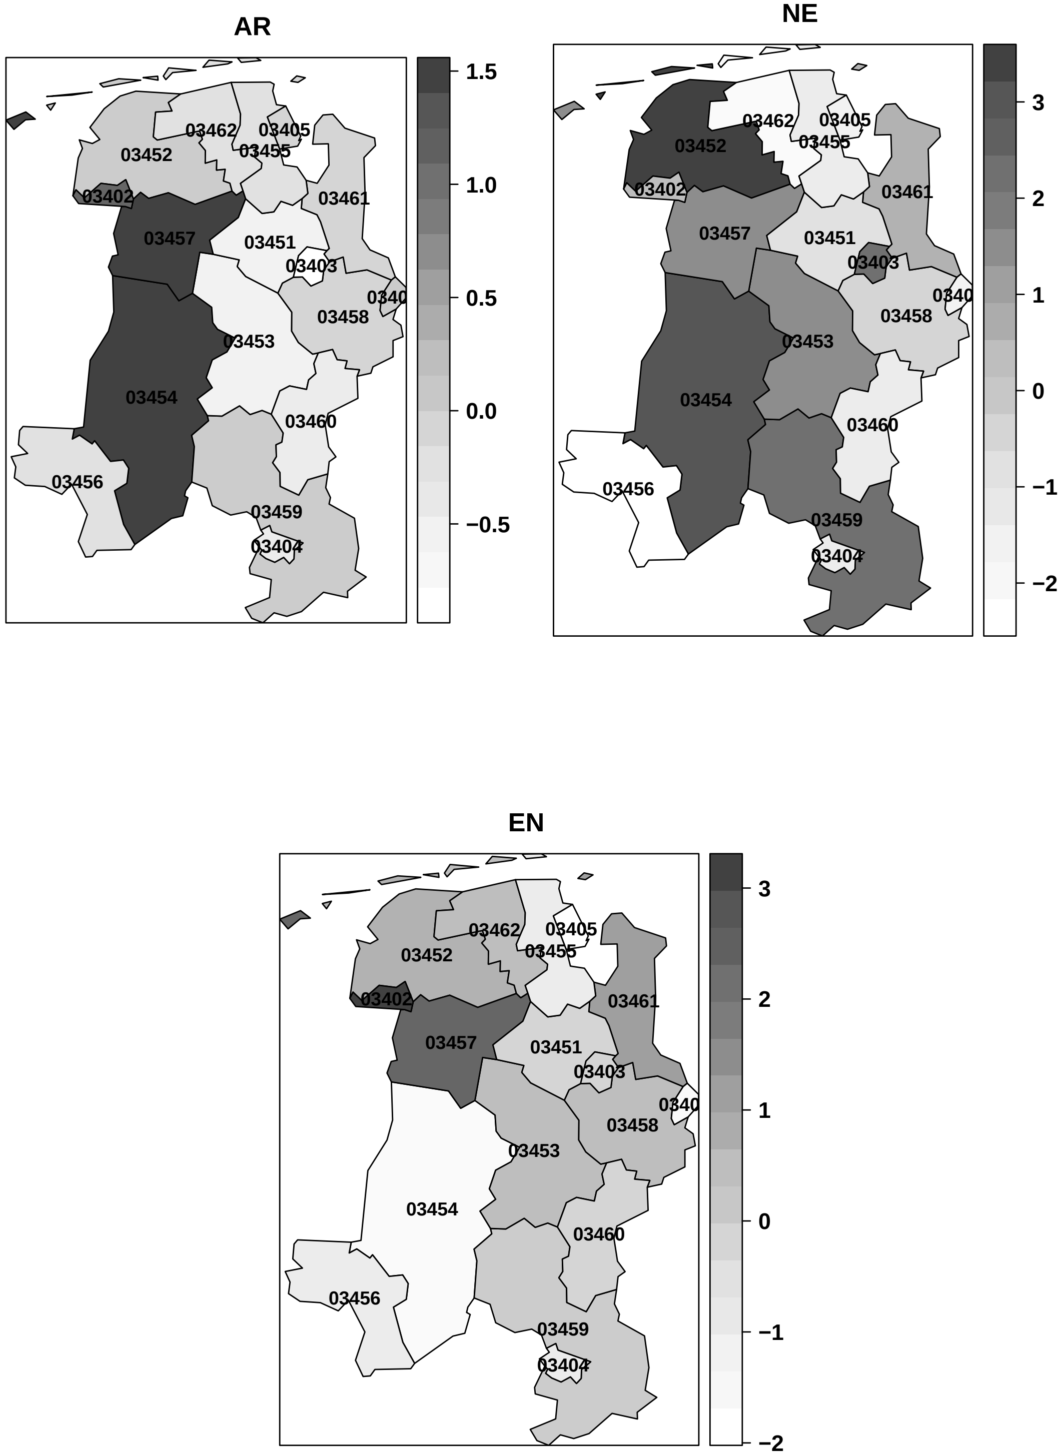


Figure 9: Posterior medians of autoregressive, neighborhood and endemic random effects $b_i^{\mathsf{AR}}$, $b_i^{\mathsf{NE}}$ and $b_i^{\mathsf{EN}}$.

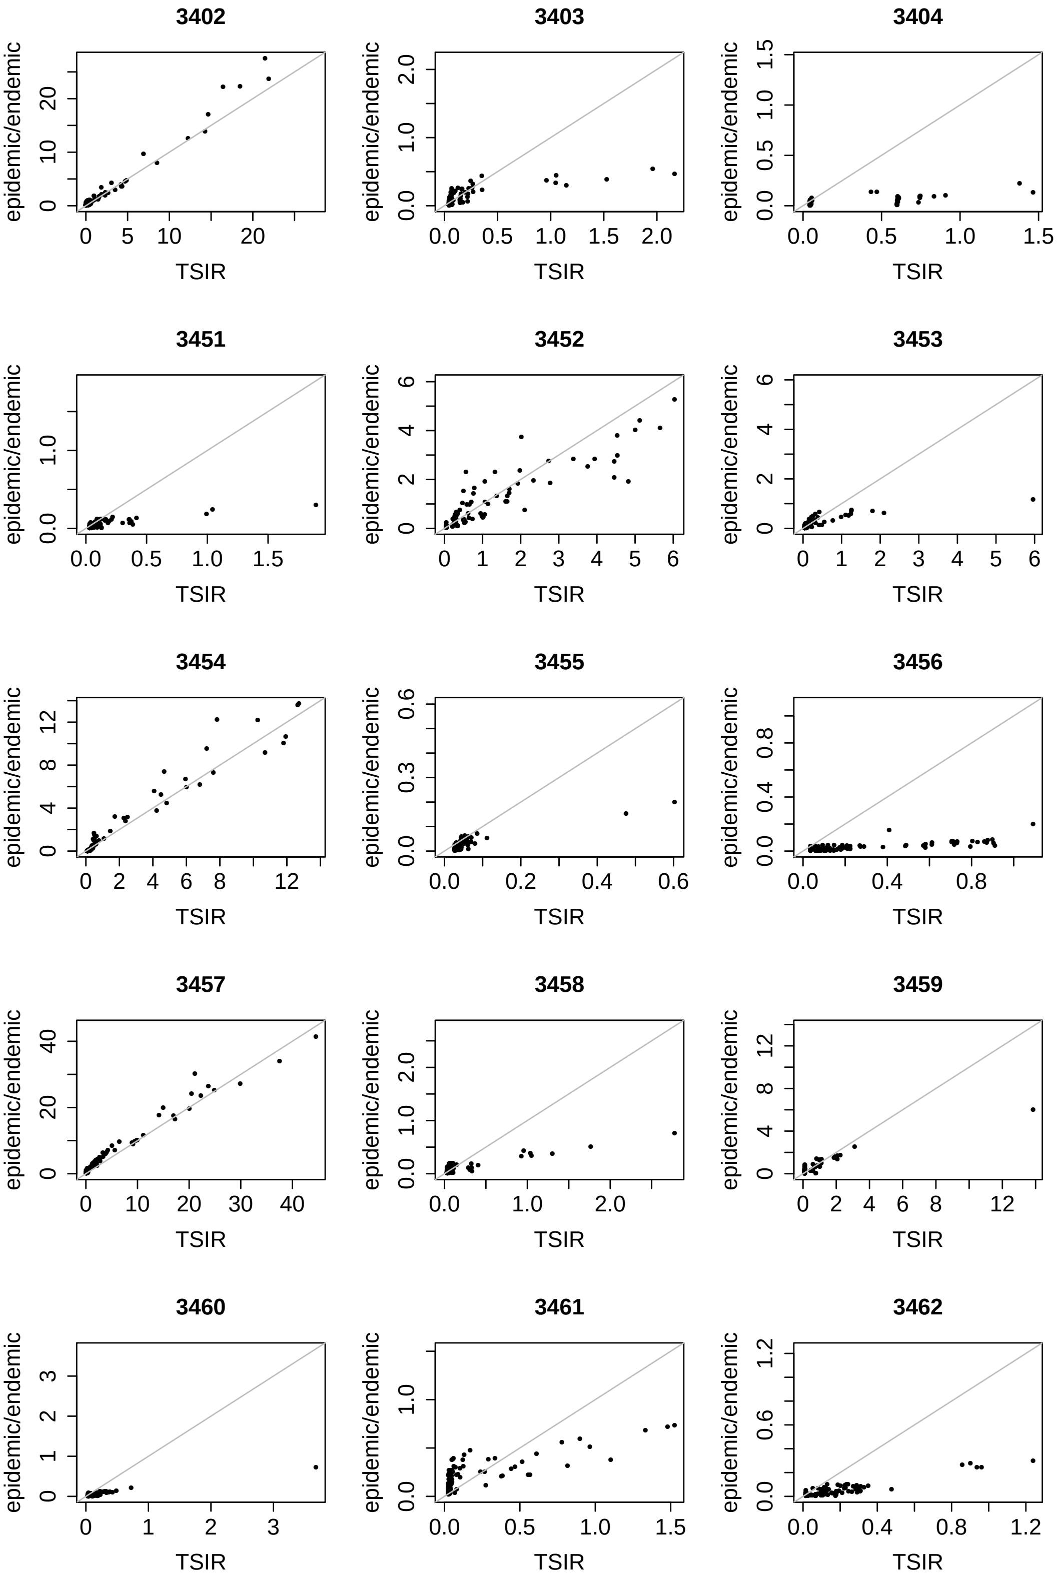


Figure 10: Posterior medians of $\mu_{it}$ under the epidemic/endemic model and the TSIR model in the 15 districts with non-zero counts.
